# Supplementary material for: Learning the kernel matrix via predictive low-rank approximations
Source: arXiv:1601.04366 source file (2016-05-09)
Supplement: Supplementary file 1 [file supplement_beta_norm_bound.tex]

\subsection{Bound on $\ell_p$ norm of primal/dual coefficients}

\emph{Proposition}. Let $\mx{\beta}_{G}$ and $\mx{\beta}_{\Phi}$ be the Ridge regression weights in the input spaces associated to matrices \mx{G} and \mx{\Phi}, respectively. Then, the following relation holds
\beq
    \|\mx{\beta}_{\Phi}\|_p \leq \|\mx{\beta}_{G}\|_p \| \mx{G}^{\dagger} \|_p \|\mx{\Phi}\|_p
\eeq

where $\cdot^{\dagger}$ denotes the Moore-Penrose pseudo-inverse, and $\| \cdot \|_p$ denotes any $\ell_p$ norm (used in a vector/matrix sense where appropriate).

\emph{Proof}. Let the Cholesky factor $\mx{G}$ be the input space associated to the regression problem. By assumption of RR, the weights $\mx{\beta}_G$ are given as some combination of the input points, given by the dual coefficients $\mx{\alpha}$:

\beq
\mx{\beta}_{G} = \mx{G}\mx{\alpha} = \mx{G}{\color{red} (\mx{G}\mx{G}^T + \lambda\mx{I})\mx{y}}
\label{e:rr_primal_g}
\eeq

The situation for the input space $\mx{\Phi}$ is analogous:
\beq
\mx{\beta}_{ \Phi } = \Phi\mx{\alpha} = \Phi{\color{red}(\mx{G}\mx{G}^T + \lambda\mx{I})\mx{y}}.
\eeq

In our case, Eq.~\ref{e:rr_primal_g} represents and underdetermined linear system of equations with dual coefficients $\mx{\alpha}$ as unknowns. One way to solve Eq.~\ref{e:rr_primal_g} for $\mx{\alpha}$ is using the pseudo-inverse $\mx{G}^{\dagger}$, yielding the minimal euclidead norm solutions. This solution would yield controllable bounds on the norm $\|\mx{\beta}_\Phi\|_p$ but would in general not be sparse.

Another option is to solve the \emph{mathing basis pursuit} problem, that will give a sparse solution with respect to $\|\mx{\alpha}\|_1$. See \url{http://spams-devel.gforge.inria.fr/} for details. The relation between the norms of primal coefficients are now less clear (however, $\|\mx{\beta}_\Phi\|_p$ would still be influenced by $\|\mx{\beta}_G\|_p$).
