# Supplementary material for: Learning the kernel matrix via predictive low-rank approximations
Source: arXiv:1601.04366 source file (2016-05-09)
Supplement: Supplementary file 2 [file supplement_greedy_low_rank_kernel.tex]

% Supplementary material to from the complete article.

\section{Supplementary material}

\subsection{Greedy low-rank approximations to the kernel matrix}

Let $\mx{K} \in \mathbb{R}^{n \times n}$ be any symmetric matrix. In this
section, we present greedy methods for low-rank approximation of form $\mx{K} =
\mx{G}\mx{G}^T$, where $\mx{G} \in \mathbb{R}^{n \times r}$ is a matrix of column
rank $r$. The problem is well known in numerical linear algebra and can be solved in
context of kernel methods with methods such as the Nystr\"om
approximation~\cite{Kumar2012,Williams2001,Li2015}, Random Fourier
Features\cite{Rahimi2007,Rahimi2009,Le2013a,Yang2014}, or direct approximation
of the kernel function~\cite{Vedaldi2012}.

\subsubsection{Incomplete Cholesky Decomposition}

Fine and Shai~\cite{Fine2001} proposed Incomplete Cholesky Decomposition (ICD)
as a modification of the original Cholesky
decomposition~\cite{golub2012matrix}.  The former reconstructs $\mx{K}$ exactly
with time complexity $O(n^3)$. ICD selects pivot columns in \mx{G} using a
greedy strategy and employs the strategy of early stopping after selecting up
to $r$ pivot columns. This results in reduction of time complexity to
$O(nr^2)$.

The algorithm starts by initializing the diagonal vector $\mx{d}(i) = \mx{K}(i,
i)$. These values represent lower bounds on the gain of the approximation error
and are updated after each iteration.  The active set $\mathcal{I}$ holds the
indices of selected pivot columns and the set
$\mathcal{J}$ holds the remaining indices. At iteration $k$, the pivot column
at index $i_k$ is selected and the current approximation is updated according
to the current residual $(\mx{K}(\mathcal{J}, k) - \mx{G}(\mathcal{J}, :)\mx{G}^T(i_k, :))$.

It is worth to note that using suitable row permutations, $\mx{G}$ can be made into
an upper-triangular matrix.  As will become clear later, we choose not to adopt
this strategy.

\begin{algorithmic}
\Function{ICD}{\mx{K}, $r$}
\State $\mx{d} \gets \text{diag(\mx{K})}$
\State $\mathcal{I} \gets \emptyset$, $\mathcal{J} \gets \{1, 2, ..., n\}$
% \State $\mathcal{J} \gets \{1, 2, ..., n\}$
\For {$k = 1 \ .. \  r$}
\State  $i_k \gets \text{argmax}(\mx{d})$
\State  $\mx{G}(i_k, k) \gets \sqrt{\mx{d}(i_k)}$

\State $\mathcal{I} \gets \mathcal{I} \cup \{i\}$, $\mathcal{J} \gets \mathcal{J} \setminus \{i\}$
% \State $\mathcal{J} \gets \mathcal{J} \setminus \{i\}$
\For{$j \notin \mathcal{J}$}
\State  $\mx{G}(j, k) \gets \frac{1}{\mx{G}(i_k, k)} (\mx{K}(j, k) - \mx{G}(j, :)\mx{G}^T(i_k, :))$
\State $\mx{d}(j) \gets \mx{d}(j) - \mx{G}(j, k)^2$
\EndFor
\EndFor
\EndFunction
\end{algorithmic}

\subsubsection{Cholesky with Side-Information}

Bach \& Jordan~\cite{Bach2005} propose Cholesky with Side-Information (CSI).
The approximation is assumed to be made in the context of supervised learning,
with available training response matrix $\mx{Y} \in\mathbb{R}^{n \times d}$,
i.e., simultaneous regression on $d$ response variables. 

The global objective function is composed of two terms: the \emph{approximation
error} of \mx{K} (ICD) and the \emph{loss} of predicting the target variables
$\mx{Y} \in\mathbb{R}^{n \times d}$ in the range space ran($\mx{G}\mx{G}^T)$. 

\beq J(\mx{G}) = \lambda \| \mx{K} - \mx{G}\mx{G}^T \|_1 + \mu\
\text{min}_{\mx{\beta} \in \mathbb{R}^{m \times d}} \| \mx{Y} -
\mx{G}\mx{\beta}\|_F^2 \label{e:bach_cost1_copy} \eeq

The $\lambda$ and $\mu$ are trade-off parameters. Setting $\mu=0$ yields the
ICD.  Observe that the right-hand term is formulated as an optimization
problem. Minimizing with respect to \mx{\beta} yields a closed form solution.
Pivots $i_k$ in Eq.~\ref{e:icd} are chosen to maximize the gain on the
objective in Eq. ~\ref{e:bach_cost1_copy}. Computing the derivative with respect to
a column $\mx{g}_i$ and maximizing yields the new pivot selection criterion:

\beq \Delta J = \| \mx{g}_i \|^2 + \| \mx{Y}^T\mx{q}_i\|^2,
\label{e:bach_gain2} \eeq where $\mx{q}_i$ is the corresponding column in the
QR decomposition.

We build on the essential contribution of ref.~\cite{Bach2005} which presents a
method to compute Eq.~\ref{e:bach_gain2} efficiently, using look-ahead
decompositions. Briefly, in ICD, the right-hand term of Eq.~\ref{e:bach_gain2},
$\| \mx{g}_i \|^2$ was estimated implicitly by using the lower-bound in
$\mx{d}$. The right-hand term is more complicated; instead of naively
recomputing its value in each iteration, the authors use the following
observation. By definition, we have

\beq \mx{g}_i = \frac{(\mx{K} - \mx{G}_k\mx{G}_k^T)(:, i)}{\sqrt{\mx{d}(i, i)}}
\eeq    

Using a emph{look-ahead} low-rank approximation, $\mx{L} = \mx{G}_{k
+\delta}\mx{G}_{k+\delta}^T$, the unknown column $\mx{g}_i$ is approximated as 

\beq \mxapp{g}_i = \frac{(\mx{L} - \mx{G}_k\mx{G}_k^T)(:, i)}{\sqrt{\mx{d}(i,
i)}} \eeq

Observe that $\mx{L} - \mx{G}_k\mx{G}_k^T =
\mx{G}_{k:k+\delta}\mx{G}_{k:k+\delta}^T.$ 
This makes the required computations more efficient, as will be illustrated more
explicitly in the derivation of our algorithm.
